# Supplementary material for: QEvict: Recoverable Quantized KV Eviction for Attention-Drift-Robust Long-Context Decoding
Source: arXiv:2608.05326 source file (2026-08-05)
Supplement: Supplementary file 1 [file B_experimental_detail.tex]

\section{Complete Experimental Details}
\label{app:experiments}

This section provides the complete evaluation protocol, baseline
configurations, memory-accounting rules, benchmark definitions, and
additional results omitted from the main paper because of space constraints.
Our experiments are designed to separate two questions. First, under a fixed
KV-memory budget, does recoverable window-level compression outperform
permanent eviction? Second, relative to methods that quantize the entire KV
cache, does selective precision allocation provide a better
performance--memory trade-off?

\subsection{Models and Inference Protocol}
\label{app:models_protocol}

We evaluate \myarch on three instruction-tuned model families:
Llama-3.1-8B-Instruct~\citep{dubey2024llama3},
Qwen2.5-7B-Instruct~\cite{hui2024qwen2}, and
Mistral-7B-Instruct-v0.2~\citep{jiang2023mistral}.
The models differ in their attention configurations, positional encodings,
and pretraining distributions, allowing us to test whether \myarch's behavior
generalizes beyond a single architecture.

\myarch is training-free and modifies only KV-cache management during
inference. It does not update model parameters, introduce task-specific
fine-tuning, or alter the output vocabulary. For each benchmark, all methods
use the same model checkpoint, tokenizer, model-specific prompt template,
maximum input length, maximum generation length, and answer post-processing
procedure. Unless otherwise stated, we use greedy decoding to remove
variation introduced by stochastic sampling.

Our evaluation covers three complementary settings:

\begin{itemize}
    \item \textbf{LongBench}~\citep{bai2024longbench} evaluates general
    long-context understanding across question answering, summarization,
    in-context learning, and synthetic retrieval tasks.
    
    \item \textbf{RULER}~\citep{hsieh2024ruler} evaluates controlled
    retrieval, aggregation, multi-hop tracing, and question answering as
    context length increases.
    
    \item \textbf{GSM8K}~\cite{mirzadeh2024gsm} evaluates whether cache compression preserves
    intermediate information required during multi-step mathematical
    reasoning.
\end{itemize}

These benchmarks stress different failure modes. LongBench measures broad
downstream quality, RULER isolates the ability to recover sparse or
distributed evidence, and GSM8K measures the stability of autoregressive
reasoning over a complete budget sweep.



\subsection{Baselines}
\label{app:baselines}

We group competing methods into \emph{eviction} and \emph{quantization}
baselines, reflecting the two principal mechanisms used to reduce KV-cache
memory. Since their technical designs are discussed in
Section~\ref{sec:related_work}, we summarize here only the methods included
in our evaluation and the role of each comparison family.

\paragraph{Eviction baselines.}
We compare \myarch against
StreamingLLM~\citep{xiao2024streamingllm},
H$_2$O~\citep{zhang2023h2o},
SnapKV~\citep{li2024snapkv},
AdaKV~\citep{feng2024adakv},
CriticalKV~\citep{feng2025criticalkv},
DefensiveKV, and
Layer-DefensiveKV~\citep{feng2025defensivekv}.
Together, these methods cover recency- and sink-based retention,
cumulative-attention heavy hitters, prompt-observation scoring,
head-adaptive budget allocation, value-aware importance estimation, and
drift-aware eviction. This group provides the primary iso-memory comparison:
all methods are evaluated under the same measured KV-cache budget, allowing
us to isolate the benefit of replacing irreversible token removal with
\myarch's recoverable window hierarchy.

\paragraph{Quantization baselines.}
Our primary global-quantization baselines are
KIVI~\citep{liu2024kivi} and
KVQuant~\citep{hooper2024kvquant}.
KIVI represents tuning-free asymmetric low-bit KV quantization, whereas
KVQuant provides a stronger sub-4-bit comparison with pre-RoPE,
outlier-aware, and non-uniform quantization mechanisms.
We additionally include ZipCache~\citep{he2024zipcache}, which assigns
precision adaptively according to token saliency.
These methods retain most or all historical states at reduced precision,
while \myarch jointly determines both residency and precision through its
full-precision, quantized, and evicted tiers. Because the methods differ in
bit width, metadata, residual regions, and retained-cache structure, we
compare them using their measured performance--memory trade-offs rather than
nominal precision alone.

\paragraph{Uncompressed reference.}
Full-KV retains the complete key and value cache in the model's native
inference datatype and serves as the upper-reference operating point for
both downstream quality and memory consumption.




\subsection{Comparison Regimes}
\label{app:comparison_regimes}

We use separate comparison protocols for eviction and quantization methods,
as identical nominal compression ratios do not imply identical physical
memory usage.

\paragraph{Eviction baselines.}
\myarch and all eviction methods are evaluated under matched measured
KV-cache budgets. For method \(\mathcal{A}\), we define the memory ratio as
\(\rho_{\mathcal{A}}=M_{\mathcal{A}}/M_{\mathrm{FullKV}}\), where
\(M_{\mathrm{FullKV}}\) is the measured memory of the complete FP16/BF16
cache. We evaluate
\(\rho_{\mathcal{A}}\in\{0.05,0.10,0.20\}\) and adjust each method's
retained-cache capacity such that its realised memory does not exceed the
target budget. This protocol isolates performance differences under equal
memory constraints.

\paragraph{Quantization baselines.}
Quantization methods differ in bit width, metadata, residual
full-precision regions, outlier storage, and packing overhead. We therefore
compare them using measured performance--memory operating points rather
than nominal precision. 


\subsection{Memory Accounting}
\label{app:memory_accounting}

For a model with \(L\) layers, \(H_{kv}\) KV heads, head dimension \(d_h\),
sequence length \(S\), and \(c_f\) bytes per element, the uncompressed
KV-cache footprint is
\begin{equation}
    M_{\mathrm{FullKV}}
    =
    2 L H_{kv} d_h S c_f,
    \label{eq:appendix_fullkv_memory}
\end{equation}
where the factor of two accounts for keys and values.

We account for all persistent cache-related storage. For eviction baselines,
this includes retained key--value tensors and method-specific state required
for selection. For quantization baselines, it includes packed codes,
quantization parameters, residual full-precision regions, outlier storage,
and persistent indexing metadata. For \myarch, the measured footprint is: 

\begin{equation}
\begin{aligned}
    M_{\mathrm{QEvict}}
    =\;&
    M_{\mathrm{sink}}
    + M_{\mathrm{recent}}
    + M_{\mathrm{FP}}
    + M_{\mathrm{Q}} 
    + M_{\mathrm{quant\text{-}meta}}
    + M_{\mathrm{position}}
    + M_{\mathrm{ledger}},
\end{aligned}
\label{eq:appendix_QEvict_memory}
\end{equation}
where \(M_{\mathrm{Q}}\) stores packed low-bit keys and values,
\(M_{\mathrm{quant\text{-}meta}}\) stores scales and offsets, and
\(M_{\mathrm{ledger}}\) stores the persistent records required for
write-once migration. Temporary workspaces are excluded from the persistent
KV-cache budget and reported separately through peak GPU memory.

\subsection{\myarch Configuration}
\label{app:QEvict_configuration}

Unless explicitly varied, \myarch uses window size \(\Omega=8\), preserves
\(N_{\mathrm{sink}}=5\) sink tokens and
\(N_{\mathrm{recent}}=32\) recent tokens, and represents the recoverable tier
using INT2 asymmetric quantization.

Let \(B_{\mathrm{hist}}\) denote the historical budget remaining after the
protected regions are allocated. We define
\(q=B_{\mathrm{quant}}/B_{\mathrm{hist}}\), with the complementary fraction
\(1-q\) assigned to the full-precision historical tier. We use \(q=0.70\)
for LongBench, RULER, and GSM8K, prioritizing broad recoverable coverage
under constrained memory. The sensitivity to window size, tier allocation,
and quantization precision is evaluated in
Appendix~\ref{app:ablations}.
