# Supplementary material for: QEvict: Recoverable Quantized KV Eviction for Attention-Drift-Robust Long-Context Decoding
Source: arXiv:2608.05326 source file (2026-08-05)
Supplement: Supplementary file 2 [file C_longbench_evaluation.tex]

% ============================================================
% LONGBENCH
% ============================================================

\section{LongBench Evaluation}
\label{app:longbench}


\subsection{Task Families and Metrics}
\label{app:longbench_tasks}

We evaluate 14 LongBench tasks spanning five complementary forms of
long-context understanding. Table~\ref{tab:longbench_task_families}
summarizes the task composition and evaluation focus of each family.


\begin{table*}[!h]
\centering
\caption{
LongBench task families used in our evaluation.
}
\label{tab:longbench_task_families}
\small
\setlength{\tabcolsep}{5pt}
\renewcommand{\arraystretch}{1.16}

\begin{tabularx}{\textwidth}{
@{}
>{\raggedright\arraybackslash\bfseries}p{0.18\textwidth}
>{\raggedright\arraybackslash}p{0.31\textwidth}
>{\raggedright\arraybackslash}X
@{}
}
\toprule
\textbf{Task Family}
& \textbf{Datasets}
& \textbf{Brief Description} \\
\midrule

Single-Document QA
& NarrativeQA, Qasper, MultiFieldQA-en
& Evidence retrieval from one long document. \\
\addlinespace[2pt]

Multi-Document QA
& HotpotQA, 2WikiMultihopQA, MuSiQue
& Evidence retrieval and reasoning across documents. \\
\addlinespace[2pt]

Summarization
& GovReport, QMSum, MultiNews
& Coverage of information distributed across the input. \\
\addlinespace[2pt]

Few-Shot Learning
& TREC, TriviaQA, SAMSum
& Retention of demonstrations and task structure. \\
\addlinespace[2pt]

Synthetic Retrieval
& PassageCount, PassageRetrieval-en
& Controlled retrieval and counting. \\

\bottomrule
\end{tabularx}
\end{table*}


We use the official LongBench metric for each dataset and report the mean
score within each task family. Family-level reporting exposes whether a
method's gains are concentrated in a particular form of long-context
understanding rather than averaging over heterogeneous tasks.



\subsection{Eviction Comparison}
\label{app:longbench_eviction}

We evaluate all eviction baselines at \(5\%\), \(10\%\), and \(20\%\) of the
measured Full-KV memory. Where supported, protected sink and recent-token
regions are matched across methods. The main paper reports complete
task-level results for Llama-3.1-8B-Instruct~\cite{dubey2024llama3} and
Mistral-7B-Instruct-v0.2~\cite{jiang2023mistral}  in
Table~\ref{tab:longbench_eviction_two_models}, and the corresponding
Qwen2.5-7B-Instruct~\cite{hui2024qwen2} results are provided in
Table~\ref{tab:longbench_qwen_eviction}.

\subsection{Quantization Comparison}
\label{app:longbench_quantization}

We compare against KIVI~\cite{liu2024kivi} and KVQuant~\cite{hooper2024kvquant} as the primary global KV-quantization
baselines, and additionally include ZipCache~\cite{he2024zipcache} as a saliency-adaptive method. For every configuration, we report both downstream performance and measured KV-cache memory. This avoids equating nominal bit width with actual storage, which can differ because of quantization parameters, residual full-precision regions, outlier handling, and mixed-precision allocation. Results for Llama and Mistral are reported in Table~\ref{tab:longbench_combined_two_models}, while the complete Qwen comparison appears in Table~\ref{tab:longbench_qwen_eviction}.



\input{Tables/Appendix/longbench_qwen_eviction}

% \input{Tables/Appendix/longbench_mistral_eviction}
% \input{Tables/Appendix/longbench_mistral_quantization}
