# Supplementary material for: QEvict: Recoverable Quantized KV Eviction for Attention-Drift-Robust Long-Context Decoding
Source: arXiv:2608.05326 source file (2026-08-05)
Supplement: Supplementary file 3 [file C_longbench_evaluation_revised.tex]

% ============================================================
% LONGBENCH
% ============================================================

\section{LongBench Evaluation}
\label{app:longbench}

\subsection{Task Families and Metrics}
\label{app:longbench_tasks}

We evaluate 14 LongBench tasks spanning the five families summarized in
Table~\ref{tab:longbench_task_families}.


We use the official metric for each dataset and report both task-level scores
and family-level means.

\subsection{Eviction Comparison}
\label{app:longbench_eviction}

Following Appendix~\ref{app:comparison_regimes}, all eviction methods are
evaluated at measured KV-memory budgets of \(5\%\), \(10\%\), and \(20\%\).
Protected sink and recent regions are matched where supported. Complete
task-level results for Llama-3.1-8B-Instruct~\citep{dubey2024llama3} and
Mistral-7B-Instruct-v0.2~\citep{jiang2023mistral} appear in
Table~\ref{tab:longbench_eviction_two_models}; corresponding
Qwen2.5-7B-Instruct~\citep{hui2024qwen2} results are reported in
Table~\ref{tab:longbench_qwen_eviction}.

\subsection{Quantization Comparison}
\label{app:longbench_quantization}

We compare \myarch with KIVI~\citep{liu2024kivi},
KVQuant~\citep{hooper2024kvquant}, and
ZipCache~\citep{he2024zipcache} at their measured memory operating points.
Llama and Mistral results are reported in
Table~\ref{tab:longbench_combined_two_models}, and the Qwen results appear in
Table~\ref{tab:longbench_qwen_eviction}.

\input{Tables/Appendix/longbench_qwen_eviction}

% \input{Tables/Appendix/longbench_mistral_eviction}
% \input{Tables/Appendix/longbench_mistral_quantization}
