# Supplementary material for: QEvict: Recoverable Quantized KV Eviction for Attention-Drift-Robust Long-Context Decoding
Source: arXiv:2608.05326 source file (2026-08-05)
Supplement: Supplementary file 4 [file mistral_longbench.tex]

% ============================================================
% Add to the preamble
% ============================================================
\usepackage{booktabs}
\usepackage{multirow}
\usepackage{array}
\usepackage{graphicx}
\usepackage[table]{xcolor}

\definecolor{qevictyellow}{RGB}{255,248,210}

\newcommand{\LBbest}[1]{\textbf{#1}}
\newcommand{\LBsecond}[1]{\underline{#1}}

% Subtle vertical separator between task families
\newcolumntype{V}{
  !{\color{black!40}\vrule width 0.35pt}
}

% ============================================================
% Tables
% ============================================================
\begin{table*}[!t]
\centering

% ============================================================
% TABLE 2: Eviction baselines
% ============================================================
\caption{
LongBench results for eviction methods at 20\%, 10\%, and 5\%
KV-cache budgets. Best and second-best compressed results are
bolded and underlined.
}
\label{tab:longbench_eviction_llama}

\vspace{-1mm}

\begingroup
\fontsize{5.4}{5.9}\selectfont
\setlength{\tabcolsep}{1.8pt}
\renewcommand{\arraystretch}{0.90}

\resizebox{\textwidth}{!}{%
\begin{tabular}{@{}lVcccVcccVcccVcccVcc@{}}
\toprule

\multirow{2}{*}{\textbf{Method}} &
\multicolumn{3}{cV}{\textbf{Single-Doc QA}} &
\multicolumn{3}{cV}{\textbf{Multi-Doc QA}} &
\multicolumn{3}{cV}{\textbf{Summarization}} &
\multicolumn{3}{cV}{\textbf{Few-Shot Learning}} &
\multicolumn{2}{c}{\textbf{Synthetic}} \\

\cmidrule(lr){2-4}
\cmidrule(lr){5-7}
\cmidrule(lr){8-10}
\cmidrule(lr){11-13}
\cmidrule(lr){14-15}

&
\textbf{Nar.QA} &
\textbf{Qasper} &
\textbf{Mul.QA} &
\textbf{Hot.QA} &
\textbf{2Wi.QA} &
\textbf{Musique} &
\textbf{Gov.Re.} &
\textbf{QMSum} &
\textbf{M.News} &
\textbf{TREC} &
\textbf{Tri.QA} &
\textbf{SAMSum} &
\textbf{PCount} &
\textbf{PR-en} \\

\midrule
\multicolumn{15}{c}{\emph{Llama-3.1-8B-Instruct}} \\
\cmidrule(lr){1-15}

Full-KV
& 30.5 & 45.5 & 55.0
& 56.0 & 45.7 & 31.3
& 35.1 & 25.6 & 27.3
& 73.0 & 91.7 & 43.7
& 6.8 & 97.5 \\

% ------------------------------------------------------------
% 20% budget
% ------------------------------------------------------------
\midrule
\multicolumn{15}{c}{\textsc{20\% Budget}} \\
\cmidrule(lr){1-15}

StreamingLLM
& 19.9 & 19.6 & 24.4
& 40.5 & 20.3 & 15.1
& 27.8 & 20.3 & 22.3
& 53.5 & 89.7 & 40.0
& 4.2 & 29.5 \\

H$_2$O
& 28.5 & 33.4 & 39.1
& 47.9 & 35.2 & \LBsecond{30.0}
& \LBsecond{31.2} & 23.1 & \LBsecond{25.0}
& 63.0 & \LBbest{92.3} & 42.5
& 6.6 & 20.0 \\

SnapKV
& 20.9 & 28.3 & 29.4
& 45.7 & 30.0 & 22.8
& 27.3 & 21.6 & 22.6
& 50.0 & \LBsecond{92.2} & \LBbest{44.6}
& 6.1 & 82.0 \\

AdaKV
& 21.7 & 28.4 & 33.5
& 50.8 & 30.4 & 21.7
& 26.4 & 21.6 & 22.9
& 55.0 & 91.4 & 43.5
& 8.5 & 80.5 \\

CriticalKV
& \LBsecond{29.9} & 31.1 & 33.2
& 51.3 & 34.3 & 24.9
& 28.5 & 22.9 & 23.1
& 55.0 & 91.8 & \LBsecond{44.1}
& \LBsecond{10.1} & 95.5 \\

DefensiveKV
& 27.1 & 40.8 & 47.8
& \LBsecond{55.3} & 38.7 & 27.9
& 29.2 & 23.7 & 23.9
& 66.0 & 91.8 & 43.7
& \LBbest{10.5} & \LBsecond{99.5} \\

Layer-Def.\ KV
& 27.7 & \LBbest{44.3} & \LBsecond{50.7}
& 53.2 & \LBsecond{40.7} & 27.5
& 30.6 & \LBsecond{24.1} & 24.6
& \LBsecond{69.0} & 91.6 & 43.7
& 8.9 & \LBbest{100.0} \\

\rowcolor{qevictyellow}
\textbf{QEvict}
& \LBbest{30.5} & \LBsecond{42.5} & \LBbest{54.0}
& \LBbest{55.4} & \LBbest{46.1} & \LBbest{31.4}
& \LBbest{33.5} & \LBbest{25.3} & \LBbest{26.8}
& \LBbest{72.5} & 91.7 & 42.4
& 7.9 & \LBsecond{99.5} \\

% ------------------------------------------------------------
% 10% budget
% ------------------------------------------------------------
\midrule
\multicolumn{15}{c}{\textsc{10\% Budget}} \\
\cmidrule(lr){1-15}

StreamingLLM
& 18.2 & 16.6 & 22.8
& 34.7 & 16.6 & 11.6
& 24.7 & 18.8 & 19.8
& 51.0 & 88.8 & 38.3
& 3.3 & 16.0 \\

SnapKV
& 18.9 & 20.8 & 23.6
& 43.0 & 22.6 & 18.2
& 24.1 & 19.6 & 20.4
& 44.5 & \LBbest{92.9} & 43.0
& 6.8 & 50.0 \\

AdaKV
& 18.3 & 22.7 & 26.1
& 40.8 & 22.2 & 17.8
& 24.3 & 20.2 & 20.9
& 46.5 & 92.2 & 43.3
& \LBbest{8.8} & 47.0 \\

CriticalKV
& 25.1 & 23.4 & 26.1
& 40.3 & 25.6 & 19.7
& 25.3 & 21.0 & 20.9
& 45.5 & \LBsecond{92.5} & 42.5
& 7.7 & 65.5 \\

DefensiveKV
& 20.9 & 26.0 & 34.0
& 48.3 & 30.0 & 19.6
& 25.1 & 22.4 & 21.5
& \LBsecond{54.0} & 91.4 & \LBsecond{43.7}
& 5.5 & \LBsecond{98.0} \\

Layer-Def.\ KV
& 22.6 & 29.1 & 37.5
& 49.6 & 30.2 & 21.7
& 25.6 & 22.6 & 21.4
& 52.0 & 91.5 & \LBbest{44.0}
& \LBsecond{8.2} & \LBsecond{98.0} \\

H$_2$O
& \LBsecond{26.9} & \LBsecond{32.0} & \LBsecond{49.8}
& \LBsecond{53.4} & \LBsecond{44.4} & \LBsecond{29.2}
& \LBsecond{27.4} & \LBsecond{23.9} & \LBsecond{22.1}
& 43.5 & 91.5 & 42.3
& 6.3 & \LBbest{99.5} \\

\rowcolor{qevictyellow}
\textbf{QEvict}
& \LBbest{30.5} & \LBbest{39.1} & \LBbest{53.2}
& \LBbest{55.5} & \LBbest{46.3} & \LBbest{31.4}
& \LBbest{31.7} & \LBbest{24.5} & \LBbest{24.4}
& \LBbest{72.5} & 91.7 & 42.3
& 7.9 & \LBbest{99.5} \\

% ------------------------------------------------------------
% 5% budget
% ------------------------------------------------------------
\midrule
\multicolumn{15}{c}{\textsc{5\% Budget}} \\
\cmidrule(lr){1-15}

StreamingLLM
& 14.3 & 13.9 & 19.7
& 30.1 & 14.7 & 7.9
& 22.2 & 17.6 & 17.3
& 38.5 & 87.8 & 36.2
& 1.5 & 9.0 \\

SnapKV
& 18.3 & 15.7 & 19.8
& 36.3 & 13.4 & 13.2
& 21.6 & 18.3 & 17.8
& 34.0 & 92.0 & 42.1
& 7.1 & 22.0 \\

AdaKV
& 17.0 & 16.4 & 19.6
& 36.7 & 17.1 & 14.4
& 21.7 & 18.7 & 18.4
& 35.5 & \LBsecond{92.8} & 42.0
& \LBsecond{7.7} & 19.0 \\

CriticalKV
& 20.2 & 17.4 & 19.6
& 36.0 & 15.5 & 15.8
& 22.7 & 18.7 & 18.2
& 34.0 & 92.5 & 42.0
& 6.2 & 22.5 \\

DefensiveKV
& 20.8 & 18.1 & 21.6
& 39.8 & 19.8 & 14.2
& 23.2 & 19.5 & 18.9
& \LBsecond{43.5} & \LBbest{93.0} & \LBbest{43.2}
& 2.8 & 72.0 \\

Layer-Def.\ KV
& 19.8 & 20.1 & 21.8
& 40.9 & 19.8 & 17.8
& 22.9 & 19.7 & 18.9
& 41.5 & \LBbest{93.0} & \LBbest{43.2}
& 6.8 & \LBsecond{81.5} \\

H$_2$O
& \LBsecond{24.8} & \LBsecond{30.1} & \LBsecond{47.5}
& \LBsecond{52.4} & \LBsecond{42.3} & \LBsecond{28.4}
& \LBsecond{25.9} & \LBsecond{23.7} & \LBbest{20.9}
& 40.5 & 90.8 & 41.3
& 6.2 & \LBbest{99.5} \\

\rowcolor{qevictyellow}
\textbf{QEvict}
& \LBbest{30.3} & \LBbest{37.2} & \LBbest{51.3}
& \LBbest{55.4} & \LBbest{46.2} & \LBbest{31.5}
& \LBbest{29.0} & \LBbest{23.9} & \LBsecond{20.5}
& \LBbest{72.5} & 91.6 & \LBsecond{42.3}
& \LBbest{7.9} & \LBbest{99.5} \\

\bottomrule
\end{tabular}%
}

\endgroup

% Compact gap between the tables
\vspace{1.2mm}

% ============================================================
% TABLE 3: Quantization baselines
% ============================================================
\caption{
LongBench results for quantized KV-cache methods and QEvict
reference points. Memory ratios are approximate.
}
\label{tab:longbench_quantization_llama}

\vspace{-1mm}

\begingroup
\fontsize{5.4}{5.9}\selectfont
\setlength{\tabcolsep}{1.6pt}
\renewcommand{\arraystretch}{0.90}

\resizebox{\textwidth}{!}{%
\begin{tabular}{@{}lVcVcccVcccVcccVcccVcc@{}}
\toprule

\multirow{2}{*}{\textbf{Method}} &
\multirow{2}{*}{
  \shortstack{\textbf{KV}\\\textbf{memory}}
} &
\multicolumn{3}{cV}{\textbf{Single-Doc QA}} &
\multicolumn{3}{cV}{\textbf{Multi-Doc QA}} &
\multicolumn{3}{cV}{\textbf{Summarization}} &
\multicolumn{3}{cV}{\textbf{Few-Shot Learning}} &
\multicolumn{2}{c}{\textbf{Synthetic}} \\

\cmidrule(lr){3-5}
\cmidrule(lr){6-8}
\cmidrule(lr){9-11}
\cmidrule(lr){12-14}
\cmidrule(lr){15-16}

& &
\textbf{Nar.QA} &
\textbf{Qasper} &
\textbf{Mul.QA} &
\textbf{Hot.QA} &
\textbf{2Wi.QA} &
\textbf{Musique} &
\textbf{Gov.Re.} &
\textbf{QMSum} &
\textbf{M.News} &
\textbf{TREC} &
\textbf{Tri.QA} &
\textbf{SAMSum} &
\textbf{PCount} &
\textbf{PR-en} \\

\midrule
\multicolumn{16}{c}{\emph{Llama-3.1-8B-Instruct}} \\
\cmidrule(lr){1-16}

Full-KV
& 100\%
& 30.5 & 45.5 & 55.0
& 56.0 & 45.7 & 31.3
& 35.1 & 25.6 & 27.3
& 73.0 & 91.7 & 43.7
& 6.8 & 97.5 \\

% ------------------------------------------------------------
% QEvict rows
% ------------------------------------------------------------
\midrule
\multicolumn{16}{c}{\textsc{QEvict}} \\
\cmidrule(lr){1-16}

\rowcolor{qevictyellow}
\textbf{QEvict}
& 10\%
& \LBbest{30.5} & 39.1 & 53.2
& \LBbest{55.5} & \LBsecond{46.3} & \LBbest{31.4}
& 31.7 & 24.5 & 24.4
& \LBbest{72.5} & \LBsecond{91.7} & 42.3
& \LBbest{7.9} & \LBbest{99.5} \\

\rowcolor{qevictyellow}
\textbf{QEvict}
& 20\%
& \LBbest{30.5} & 42.5 & \LBbest{54.0}
& \LBsecond{55.4} & 46.1 & \LBbest{31.4}
& \LBbest{33.5} & \LBbest{25.3} & \LBbest{26.8}
& \LBbest{72.5} & \LBsecond{91.7} & 42.4
& \LBbest{7.9} & \LBbest{99.5} \\

% ------------------------------------------------------------
% Quantization baselines
% ------------------------------------------------------------
\midrule
\multicolumn{16}{c}{\textsc{Quantized Baselines}} \\
\cmidrule(lr){1-16}

KVQuant-2b (s1\%)
& $\sim$15\%
& 22.6 & 36.5 & 47.1
& 43.8 & 34.2 & 23.2
& 31.5 & 22.9 & 25.8
& 65.0 & 86.3 & 41.9
& 2.9 & 36.5 \\

KIVI-2b
& $\sim$19\%
& 23.7 & 36.8 & 41.1
& 44.4 & 30.0 & 21.9
& 30.5 & 24.4 & 26.0
& \LBsecond{68.0} & 87.8 & \LBbest{44.7}
& 5.3 & \LBsecond{99.0} \\

ZipCache-4b (70\%)
& $\sim$21--23\%
& 24.1 & \LBsecond{43.3} & \LBsecond{53.9}
& 47.4 & \LBbest{50.8} & 25.2
& 32.6 & 22.9 & \LBsecond{26.5}
& 21.0 & 91.0 & 20.4
& \LBsecond{7.8} & 68.5 \\

KVQuant-3b (s1\%)
& $\sim$22\%
& \LBsecond{28.6} & \LBbest{44.3} & 53.4
& 53.9 & 42.7 & \LBsecond{28.0}
& \LBsecond{33.4} & \LBsecond{25.0} & \LBsecond{26.5}
& \LBbest{72.5} & \LBbest{92.0} & \LBsecond{44.6}
& 5.4 & \LBbest{99.5} \\

\bottomrule
\end{tabular}%
}

\endgroup
\end{table*}
